# Supplementary material for: Online Calibrated and Conformal Prediction Improves Bayesian Optimization
Source: arXiv:2112.04620 source file (2024-06-25)
Supplement: Supplementary file 2 [file supplement-main-old.tex]

\documentclass{uai2023} % for initial submission
\usepackage[ruled,vlined]{algorithm2e}
\usepackage{subfigure}
\usepackage{multirow}
% to compile a preprint version, e.g., for submission to arXiv, add add the
% [preprint] option:
%     \usepackage[preprint]{neurips_2021}

% to compile a camera-ready version, add the [final] option, e.g.:
%     \usepackage[final]{neurips_2021}

% to avoid loading the natbib package, add option nonatbib:
%    \usepackage[nonatbib]{neurips_2021}

\usepackage[utf8]{inputenc} % allow utf-8 input
\usepackage[T1]{fontenc}    % use 8-bit T1 fonts
\usepackage{hyperref}       % hyperlinks
\usepackage{url}            % simple URL typesetting
\usepackage{booktabs}       % professional-quality tables
\usepackage{amsfonts}       % blackboard math symbols
\usepackage{nicefrac}       % compact symbols for 1/2, etc.
\usepackage{microtype}      % microtypography
\usepackage{xcolor}         % colors
\usepackage{graphicx}
\usepackage{amsmath, nccmath}
\usepackage{amsthm}
\usepackage{float}
\usepackage[english]{babel}
\usepackage{caption}
%\usepackage{subcaption}
\usepackage{natbib}
    \bibliographystyle{plainnat}
    \renewcommand{\bibsection}{\section*{References}}
\hyphenpenalty 10000
\exhyphenpenalty 10000

\newtheorem{theorem}{Theorem}
\newtheorem{lemma}{Lemma}
\newtheorem{proposition}{Proposition}
\newtheorem{corollary}{Corollary}

\usepackage{xr} 
\externaldocument{main}

%% Provided macros
% \smaller: Because the class footnote size is essentially LaTeX's \small,
%           redefining \footnotesize, we provide the original \footnotesize
%           using this macro.
%           (Use only sparingly, e.g., in drawings, as it is quite small.)

%% Self-defined macros
\newcommand{\swap}[3][-]{#3#1#2} % just an example

\title{Calibrated Uncertainty Estimation Improves Bayesian Optimization (Supplementary Material)}
\author[1]{Shachi Deshpande}
\author[1]{Volodymyr Kuleshov}
% Add affiliations after the authors
\affil[1]{%
    Computer Science Dept.\\
    Cornell University and Cornell Tech\\
    Pittsburgh, Pennsylvania, USA
}
  \begin{document}
  \onecolumn
\maketitle
\nopagebreak
% \maketitle

\input{9_appendix}
\bibliography{bibliography}
\end{document}
